# Supplementary material for: DPCube: Differentially Private Histogram Release through Multidimensional Partitioning
Source: arXiv:1202.5358 source file (2012-02-24)
Supplement: Supplementary file 1 [file Appendix_F.pdf]

# APPENDIX F

## The IEEEeqnarray Commands

### *(Optional---for advanced users)*

Virtually all LaTeX alignment commands such as `\eqnarray`, `\array`, and `\tabular` are based on the TeX command `\halign`. LaTeX's goal of simplifying the use of `\halign` is noble. However, in hiding much of the lower level interface, a fair degree of flexibility is lost. This has resulted in the development of several packages such as amsmath [7], array.sty [13], and the MDW tools [8], each of which provides much more powerful alignment structures.

IEEEtran also provides its own unique set of alignment tools which are known as the IEEEeqnarray family. The design philosophy of the IEEEeqnarray family is to provide a LaTeX alignment interface that is based more closely on the underlying `\halign`, but to couple this with high-level column definition management and automated preamble building mechanisms (which are tedious to do in TeX). As a result, the IEEEeqnarray family of commands are flexible enough to be almost universal replacements for all the other LaTeX commands for producing multiline equations and aligned box structures such as matrices and tables of text and/or mathematics. Because the user is shielded less from the `\halign` underpinnings, the rules of operation are more involved. So, the IEEEeqnarray commands are aimed primarily toward the more advanced LaTeX users.

The use of the IEEEeqnarray family of tools described in this section is totally *optional*. The IEEEeqnarray code is self-contained and does not depend on other alignment packages—which can be used along side, or in place of, it. The IEEEtrantools.sty package (See Appendix C.2) is available for those who wish to use the IEEEeqnarray family outside of IEEEtran.cls.

### F.1 IEEEeqnarray

The IEEEeqnarray environment is for multiline equations that occupy the entire column. It is used in much the same way as `\eqnarray`, but with two additional arguments, one of which is mandatory and the other is optional:

```
\begin{IEEEeqnarray}[decl]{cols}
.
\end{IEEEeqnarray}
```

The optional argument is for commands that are to be executed within the environment, but before the alignment actually begins. This is just like the local control of the IEEEtran IED list environments. There is also a global control, `\IEEEeqnarraydecl`, which is executed just prior to the local control. By default, `\IEEEeqnarraydecl` is defined to be \relax. As mentioned in the Section 10, users should be careful not to allow unwanted spaces to occur in these controls because such things will appear just before the IEEEeqnarray structure. Furthermore, remember that, to prevent the LaTeX parser from becoming confused, the contents of an optional argument must be enclosed in braces if the argument contains commands with optional arguments.

The mandatory argument *cols* contains the column and intercolumn separator spacing ("intercolumn tabskip glue" in TeX speak) type specifiers. Column types are identified by letters. Several predefined column types are available as shown in Table 4. There are two kinds of glue types. Predefined glue types are indicated by various punctuation marks as shown in Table 5. User defined glue types are indicated by numbers.

The rules for placing these specifiers are as follows:

1. No two glue specifiers can appear next to each other—they are not additive and must be separated from each other by at least one column specifier.
2. Zero intercolumn spacing will be assumed between back-to-back column specifiers.
3. Because of rule one, back-to-back numerals will be considered as being a single glue specified by the numerical value represented by all the digits.
4. A multiletter column specifier can be accessed by enclosing the letters within braces (otherwise, it would be interpreted as being several single letter column specifiers). Because of rule three, braces are not needed around multidigit glue specifiers.
5. There must be at least one column specifier, but there is no fixed upper limit of how many columns can be supported
6. For `\IEEEeqnarray`, "+" centering glue will be assumed at each end of the cols specification if no column glue is specified there. This results in a centered structure like `\eqnarray` (the 1,000pt minus 1,000pt glue on each side "compresses" as needed from each side of the main text column to center that which is between).

Also, `\IEEEeqnarray` automatically adds a hidden column for equation numbers to the right of the last specified column. Currently, there is no support for equation numbers on the left side.[1]

### F.2 Defining Column Types

New column types are defined with the

`\IEEEeqnarraydefcol{`*`col_id`*`}{`*`predef`*`}{`*`postdef`*`}`

command. The *`col_id`* argument contains the name of the column specifier which should consist only of one or more letters. A given column specifier, even the predefined ones, can be redefined at will without warning or error.[2] The predef argument contains the commands that will be inserted before each cell in the column. The postdef argument contains the commands that will be inserted after each cell in the column. For example,

```
\IEEEeqnarraydefcol{g}{\hfil$\clubsuit$}{$\dia
mondsuit$\hfil}
```

[1] This is not to say that it's impossible with the existing capability, just ugly.
[2] Thus, allowing new predefined column types to be added without breaking existing code.

TABLE 4
IEEEeqnarray Predefined Column Types

| I.D. | Description | I.D. | Description |
|---|---|---|---|
| l | left math | v | vertical rule |
| c | centered math | vv | two vertical rules |
| r | right math | V | double vertical rule |
| L | left math with ords | VV | two double vertical rules |
| C | centered math with ords | h | horizontal rule |
| R | right math with ords | H | double horizontal rule |
| s | left text | x | empty |
| t | centered text | X | empty math |
| u | right text | | |

**Note:** S, T, U, p, and P are likely to be used in future versions.

TABLE 5
IEEEeqnarray Predefined Column Separation (Glue) Types

| I.D. | Width* | I.D. | Width |
|---|---|---|---|
| ! | −1/6 em | . | 0.5\arraycolsep |
| , | 1/6 em | / | 1.0\arraycolsep |
| : | 2/9 em | ? | 2.0\arraycolsep |
| ; | 5/18 em | * | 0pt plus 1fil |
| ' | 1 em | + | 1000pt minus 1000pt |
| " | 2 em | − | 0pt |

*All em values are referenced to the math font.
1 em = \quad, 2 em = \qquad

Will define a "g" text column which will place club and diamond suit symbols on either side of a cell's contents and center the respective structure within the cell, e.g.,

```
\hfil$\clubsuit$Hello$\diamondsuit$\hfil
```

Using \hfil to control cell alignment allows the user to override the column alignment on a cell-by-cell basis by placing the infinitely more stretchable \hfill on one or both sides of a cell's contents. \hfill can even be placed between items in a cell to force them apart and against the "cell walls." The IEEEeqnarray predefined columns are designed to allow user overrides via \hfill whenever possible (even for the math mode cells).

Please note that TeX will not allow unmatched braces within the arguments of commands. If braces are needed, such as for the argument of a command, they will have to be provided within the cells themselves. For example,

```
\IEEEeqnarraydefcol{myp}{\parbox[c]{0.5in}}{}
\begin{IEEEeqnarraybox}{{myp}c}
{first\\second}&\alpha\\
&\beta%
\end{IEEEeqnarraybox}
```

defines a column type named "myp" that will place text within a 0.5inch wide parbox which is centered on the cell's baseline. Note that because the column type name consists of more than one letter, it has to be enclosed within an extra set of braces in the column specifications or else it would be interpreted as three adjacent columns "m," "y," and "p." Also, the contents of the cell must be enclosed within braces so that 1) the \parbox command sees the entire contents as its argument and 2) the newline within the parbox will not be interpreted as being the end of the alignment row. Be aware that it can happen that a column is given an empty cell, such as in the second row in the example, or when entering blank separator rows. When this happens, a \relax will appear in the column which will be acquired as the command's argument. Therefore, commands in column definitions that acquire arguments from the cells should not choke if fed \relax.

For reference, the definitions of the predefined column types are shown here:

```
% math
\IEEEeqnarraydefcol{l}{$\IEEEeqnarraymathstyle
}{$\hfil}
\IEEEeqnarraydefcol{c}{\hfil$\IEEEeqnarraymath
style}{$\hfil}
\IEEEeqnarraydefcol{r}{\hfil$\IEEEeqnarraymath
style}{$}
\IEEEeqnarraydefcol{L}{$\IEEEeqnarraymathstyle
{}}{{}$\hfil}
\IEEEeqnarraydefcol{C}{\hfil$\IEEEeqnarraymath
style{}}{{}$\hfil}
\IEEEeqnarraydefcol{R}{\hfil$\IEEEeqnarraymath
style{}}{{}$}
% text
\IEEEeqnarraydefcol{s}{\IEEEeqnarraytextstyle}
{\hfil}
\IEEEeqnarraydefcol{t}{\hfil\IEEEeqnarraytexts
tyle}{\hfil}
\IEEEeqnarraydefcol{u}{\hfil\IEEEeqnarraytexts
tyle}{}
% vertical rules
\IEEEeqnarraydefcol{v}{}{\vrule
width\arrayrulewidth}
\IEEEeqnarraydefcol{vv}{\vrule
width\arrayrulewidth\hfil}
{\hfil\vrule width\arrayrulewidth}
\IEEEeqnarraydefcol{V}{}
{\vrule
width\arrayrulewidth\hskip\doublerulesep\vrule
width\arrayrulewidth}
\IEEEeqnarraydefcol{VV}
{\vrule
width\arrayrulewidth\hskip\doublerulesep\vrule
width\arrayrulewidth\hfil}{\hfil\vrule
width\arrayrulewidth\hskip
\doublerulesep\vrule width\arrayrulewidth}
% horizontal rules
\IEEEeqnarraydefcol{h}{}{\leaders\hrule
height\arrayrulewidth\hfil}
\IEEEeqnarraydefcol{H}{}
{\leaders\vbox{\hrule
width\arrayrulewidth\vskip\doublerulesep\hrule
width
\arrayrulewidth}\hfil}
```

```
% plain
\IEEEeqnarraydefcol{x}{}{}
\IEEEeqnarraydefcol{X}{$}{$}
```

Note the inclusion of the commands `\IEEEeqnarraymathstyle` and `\IEEEeqnarraytextstyle` in the math and text columns, respectively. These commands allow the user to control the style of all of the math and text columns. However, because the changes apply to all the columns, the user will have to define new column types if different styles are needed in the same alignment (or different styles can be manually specified in each cell). The default definitions for these commands are

```
\newcommand{\IEEEeqnarraymathstyle}{\displaystyle}
\newcommand{\IEEEeqnarraytextstyle}{\relax}
```

which allows the text columns to be in whatever style was in effect when the alignment was started and the default math style will be in display style, but can be easily changed as needed. e.g.,

```
\begin{IEEEeqnarray}[\renewcommand{\IEEEeqnarraymathstyle}
{\scriptstyle}]{rCl}
```

will result in script style math columns.

The columns relating to vertical and horizontal lines will be discussed in Appendix F.11 as they are typically used only when producing tables.

The "x" and "X" columns are basic empty text and math mode columns without any formatting or style controls.

### F.3 Defining Glue Types

New column separation glue types are defined with the

```
\IEEEeqnarraydefcolsep{colsep_id}{def}
```

command. The `colsep_id` argument contains the number of the column separation glue specifier which should consist only of numerals. Different glue type names must have different numerical values. (Don't get too cute—"007" is identical to "7.") User defined column glue specifiers can be redefined at will without warning or error. The def argument contains the width of the given glue type. Widths may be specified as absolute values or reference length commands:

```
\IEEEeqnarraydefcolsep{9}{10pt}
\IEEEeqnarraydefcolsep{11}{2\tabcolsep}
```

The glue type widths are *not* evaluated when defined, but are evaluated each time they are actually referenced as IEEEeqnarray column specifiers. Thus, for the second definition in the example above, if `\tabcolsep` were to be revised after the glue type was defined, the revised value would be what is used.

Rubber lengths are allowed too. The fact that the centering glue "+" is a known value can be exploited to achieve some interesting effects. For example,

```
\IEEEeqnarraydefcolsep{17}{200pt minus 200pt}
```

will produce a column separation glue that is always 1/5 of the width of the distance from the equation sides to the ends of the main text columns. And, of course, "+" can be used as needed to produce groups of equally spaced equations as in amsmath's `\align`:

```
\begin{IEEEeqnarray}{Rl+Rl+Rl}
```

### F.4 A Simple Example of Use

The example in the Section 8 can be implemented using `\IEEEeqnarray` via

```
\begin{IEEEeqnarray}{rCl}
Z&=&x_1 + x_2 + x_3 + x_4 + x_5 +
x_6\IEEEnonumber\\
&&+\:a + b%
\end{IEEEeqnarray}
```

As shown in Table 4, the "C" column type is a centered math mode column with empty ords ("{}") on either side. So, there is no need to place empty ords around the equal sign. As with `\eqnarray`, the `&` separate the column cells and are where the intercolumn separation glue will appear (when nonzero).

Note the presence of the `%` at the end of the second row. TeX does *not* ignore spaces that occur *before* commands or `&` column delimiters, but does ignore those that occur *after*. Most LaTeX alignment implementations shield the user from this behavior by removing all spacing previous to `&`, `\\`, and `\end`. The IEEEeqnarray family does not do this! So, it is important to prevent spaces (including implied ones at the end of lines) from occurring before such commands unless they are wanted. One should suspect this problem if there is an unexplained offset within a column. In the given example, unwanted spacing is not an issue because end spacing is ignored in math mode anyway. However, it would be an issue if the columns used text mode instead.

Alternatively, one could use a two column form:

```
\begin{IEEEeqnarray}{Rl}
Z=&x_1 + x_2 + x_3 + x_4 + x_5 +
x_6\IEEEnonumber\\
&+\:a + b%
\end{IEEEeqnarray}
```

### F.5 Equation Numbering

Like `\eqnarray`, `\IEEEeqnarray` has a "star form," `\IEEEeqnarray*`, which does not place equation numbers at the end of each row by default. The default behavior of individual rows can be overridden by placing the commands `\IEEEnonumber` or `\IEEEyesnumber` as needed in the last

column.[3] `\IEEEeqnarray` also provides a `\IEEEyessubnumber` which can be used to enable a subequation number for the given line:

```
&+\:a +
b\IEEEyessubnumber\label{myfirstsubeqn}\\
```

Note that labels for subequations must be placed *after* the `\IEEEyessubnumber` command because, prior to that point, the label will reference the equation number *that would have been used* if there had not been a request for a subnumber. To support this feature, IEEEtran defines its own IEEEsubequation counter (reset with changes to `equation`) and `\theIEEEsubequation` command.[4] The first line without an `\IEEEyessubnumber` will revert back to conventional equation numbering. Currently, there is no support for subequation numbering to be the default for all the lines. So, users will have to call `\IEEEyessubnumber` every time a subequation number is needed.

Please be aware that `\IEEEeqnarray`, like `\eqnarray`, will, if the equation is long enough, overwrite the equation number without warning![5] For cases when this happens, users can insert a `\IEEEeqnarraynumspace` command at the end of the line (after any `\IEEEyessubnumber` if used) which will insert a space equal in width to the displayed equation number:

```
... + x_z
\IEEEyessubnumber\IEEEeqnarraynumspace\\
```

As a result, the entire multiline equation will be slightly shifted to the left. IEEE often does the same thing in its journals when confronted by this situation. If an overfull hbox results, the offending equation line will have to be further divided.

## F.6 Extra Vertical Spacing and Page Breaks

Like `\eqnarray`, `\IEEEeqnarray`'s `\\` command supports a star form which inhibits page breaks at the given line as well as an optional extra vertical spacing argument:

```
&+\:a + b\\*[5pt]
```

Users are reminded from Section 8 that amsmath will configure LaTeX to disallow page breaks within multiline equations—including those made by `\IEEEeqnarray` because it also honors the value of \interdisplaylinepenalty.

Also, like `\eqnarray`, `\IEEEeqnarray` normally places a small amount of extra spacing (as specified by the length command `\jot`) between lines to "open up" equations as well as to prevent large symbols from coming to close to the lines above them.

## F.7 IEEEeqnarraybox

`\IEEEeqnarray` is not suitable for producing structures such as matrices and tables because it must have exclusive access to the main text column and cannot be nested within other structures. For these applications, the `\IEEEeqnarraybox` command is provided. `\IEEEeqnarraybox` differs from `\IEEEeqnarray` in the following ways:

1. The entire contents are wrapped within a box and, therefore, can be nested within other display or alignment structures (such as `\equation`, `\IEEE eqnarray`, or even another `\IEEEeqnarraybox`). Note that, like all box structures, page breaks are *not* allowed between the rows of an `\IEEEeqnarraybox`.
2. The default glue at the outer ends of the first and last columns is 0pt ("-"), not "+" centering glue as with `\IEEEeqnarray`.
3. No automatic (hidden) equation number column is provided.
4. The star form "`\IEEEeqnarraybox*`" turns off the extra `\jot` vertical spacing after each row.
5. `\IEEEeqnarrayboxdecl` is the global control.

Two subforms are provided: `\IEEEeqnarrayboxm`, which is for use within math modes and is analogous to `\array` and `\IEEEeqnarrayboxt`, which is for use within text modes and is analogous to `\tabular`. If called via `\IEEEeqnarraybox`, the current math/text mode will be auto-detected and the proper subform will automatically be selected. Therefore, `\IEEEeqnarraybox` can replace `\array` as well as `\tabular`.

The syntax for `\IEEEeqnarraybox` is similar to `\IEEEeqnarray`, but with two additional optional arguments:

```
\begin{IEEEeqnarraybox}[decl][pos][width]{cols
}
.
\end{IEEEeqnarraybox}
```

The *pos* argument can be one of `t`, `c`, or `b` to control where the box will be vertically aligned relative to the current baseline: `t` at the top row, `c` at the center,[6] `b` at the bottom row. The default is `b`.

The *width* argument specifies the width the box. **Warning**: If a width is specified, there *must* be one or more rubber lengths in the intercolumn glue specifiers (such as that of "*" or "+") so that the box can be sized as needed. If there is no such glue, or the glue provided cannot stretch/shrink enough as needed, the box cannot be sized to width and an underfull or overfull hbox error will result. If no width argument is provided, the box will be set to its

[3] The aliases `\nonumber` and `\yesnumber` are also provided. However, their use is not recommended because some packages (such as MDW tools) redefine them in an IEEEeqnarray incompatible way.

[4] What is actually displayed is the `\theIEEEsubequationdis` command.

[5] This behavior is extremely difficult to avoid if the equation line is to remain centered irrespective of the width of the equation number—without even considering the subjective question of how close is too close for any given case.

[6] Centering is actually done along the "math axis," not exactly on the text baseline (but quite close to it). Most LaTeX users are not aware of this minor distinction.

natural width (and the use of rubber inter-column glue will not be required).

`\IEEEeqnarraybox` uses the same column and glue type specifiers/definitions as `\IEEEeqnarray`.

### F.8 Line Spacing in LaTeX

Before discussing some of the more advanced aspects of vertical spacing control in the IEEEeqnarray family, it is important to review the details of LaTeX's line spacing algorithm. Normally, baselines are separated by the amount given by the length command `\baselineskip`. With each change in font size, `\baselineskip` is reset to the default value for that font size (multiplied by `\baselinestretch`). Then, the value of `\baselineskip` is saved to the length variable `\normalbaselineskip` (so that the normal value can be later referenced even if `\baselineskip` is set to another value by the user). However, if the top of a line ever gets closer than `\lineskiplimit` to the bottom of the line above it, the use of `\baselineskip` will be suspended and \lineskip spacing will be placed between the two lines.[7]

This system works well for text. However, for mathematics, whose symbols have a much higher dynamic range of heights and depths, it is usually better to go ahead and always add an extra fixed amount of space (`\jot`) as mentioned in the Appendix F.6.

When the IEEEeqnarray family is loaded, two new length commands are defined: `\normaljot` and `\normalsizebaselineskip` which store the nominal values of `\jot`[8] and the `\baselineskip` of the normalsize font, respectively, so that they can be always be referred to even if other values are currently being used.

At the start of `\IEEEeqnarray/box`, but before the local or global controls, the following initialization takes place:

```
\lineskip=0pt
\lineskiplimit=0pt
\baselineskip=\normalbaselineskip
\jot=\normaljot
```

Thus, `\baselineskip` is set to the normal value for the current font, `\jot` is restored to its nominal value and the `\lineskiplimit` system is disabled.[9]

This system is designed to better facilitate nested IEEEeqnarraybox structures as well as to help prevent the user from encountering seemingly uncontrollable spacing behavior (e.g., "How *do* I get rid of that unwanted space?!").

### F.9 The IEEEeqnarray Strut System

When creating tables, especially tables with vertical rules, vertical space between the rows of the table is not generally desirable because such space will suspend the column cell definitions and "cut across" any vertical rules that may be present. Yet, there must be a way to keep rows adequately spaced apart. To solve this problem, the IEEEeqnarray/box commands provide an integrated system to manage struts[10] contained in a hidden column on the right end of each IEEEeqnarray/box structure.

The struts in each row will be set to a default strut height and depth. Normally, the default strut height and depth are initialized to zero, so the struts will effectively not be present. The user can set the default strut values via the

```
\IEEEeqnarraystrutsize{height}{depth}[decl]
```

command which can be placed in a local or global control. The optional argument is for commands which will be executed prior to the evaluation of the height and depth arguments. Thus,

```
\IEEEeqnarraystrutsize{0.5\baselineskip}{}[\large]
```

will set the default strut height to half the baselineskip used by the large font size, even if the current baselineskip (and/or font size) is different. The commands which are executed within the optional argument are contained within their own environment so as not to have any effects outside of the `\IEEEeqnarraystrutsize` command. For mimicking the action of `\baselineskip`, the typically recommended height and depth of struts is 70 and 30 percent, respectively, of `\normalbaselineskip`.[11] `\IEEEeqnarraystrutsize` will assume these values if its height and/or depth arguments are left blank, e.g., in the previous example, the strut *depth* will be set to 30 percent of `\normalbaselineskip` for the large font size.

There is also a

```
\IEEEeqnarraystrutsizeadd{height}{depth}[decl]
```

command which will *add* to the current default strut values and can be used much like the `\extrarowheight` parameter of the array.sty package. Empty arguments are assumed to be 0pt.

`\IEEEeqnarraystrutsize` and `\IEEEeqnarraystrutsizeadd` can also be used at the *end of the last* column to alter the strut size used for a particular row (the default strut values of the other rows will not be affected).

There is also a

```
\IEEEstrut[height][depth][decl]
```

which produces a strut. It can be used whenever a "manual" strut is needed—even outside the `\IEEEeqnarray/box` environments. If a height or depth argument is not provided (or empty), then these will be assumed in the same way as `\IEEEeqnarraystrutsize` does.

---

[7] Within IEEEtran.cls, `\lineskiplimit` and `\lineskip` are zero—if things get too close it is the author's responsibility to correct the problem without having IEEEtran.cls second guessing the author's intent.
[8] Within IEEEtran.cls, the nominal value of `\jot` is 25 percent of the baselineskip for the normalsize font.
[9] As long as rows cannot be of negative height.

[10] "Struts" are vertical rules of zero width, but of finite height.
[11] Note that this *not* the *normalsize* baselineskip, but the normal baselineskip for the current font.

For diagnostic purposes (in order to see if any row objects exceed the height of the struts), the command `\IEEEvisiblestrutstrue` can be placed with an `\IEEEeqnarray/box` or `\IEEEstrut` control to make the struts visible.

When using `\IEEEeqnarraybox` to produce tables that contain vertical lines, it is usually desirable to shutdown the `\baselineskip` system and switch over to pure strut spacing. The following command sequence, placed within a local or global control, will serve this purpose:

```
\IEEEeqnarraystrutsize{0.7\normalbaselineskip}
{0.3\normalbaselineskip}
[\relax]
\setlength{\baselineskip}{0pt}%
\setlength{\lineskip}{0pt}%
\setlength{\lineskiplimit}{0pt}%
\setlength{\jot}{0pt}%
```

Note the use of "`%`" to prevent the ends of the lines that end in braces from being interpreted as unwanted spaces. Because of the frequent need to call this sequence, the IEEEeqnarray family provides the `\IEEEeqnarraystrutmode` command which does the same thing.

### F.10 Overriding Column Types

Within a row, one or more column types can be overridden by placing the command

`\IEEEmulticol{`*`num_cols`*`}{`*`col_type`*`}{`*`text`*`}`

as the *very first* command in a cell. This command is the IEEEeqnarray equivalent of `\multicolumn`. The first argument is the number of columns to override (cutting through any intercolumn glues as needed). The second argument is the column type specifier to use. The third argument contains the cell text. The third argument will have to be enclosed within an extra set of braces if the column type is to acquire it as an argument—as was done with the "myp" parbox column type in the example earlier in this Appendix E.2.

There is also the `\IEEEeqnarrayomit` command which, when used as the very first command in a cell, will suspend the use of the normal column type for that cell. This is somewhat like a quicker version of `\IEEEeqnarraymulticol{1}{x}{}`.

Users are cautioned not to use commands like these (e.g., `\multicolumn`) that are designed for other alignment environments.[12]

### F.11 Predefined Column Types for Rules

Several of the predefined column types produce vertical or horizontal lines. Note that, in the IEEEeqnarray family, rules are declared and treated as normal column types—they are not hidden. Although this approach may increase the number of columns the user has to keep track of, especially when creating tables, it does offer a great deal of flexibility by allowing the user to override, or otherwise manipulate, any column type (including those that produce rules) at will.

All of the predefined rule column types use the `\arrayrulewidth` length to determine the line thickness and `\doublerulesep` for the spacing of double rules.

The "`v`" column type produces a vertical rule and "`vv`" produces two back-to-back vertical rules which will appear as one rule of twice the normal thickness. "`V`" produces a double vertical rule with `\doublerulesep` spacing between its two lines. "`VV`" produces two back-to-back double vertical rules which will appear to be three vertical rules, the middle one of which being twice as thick as the other two. It is possible to "spread apart" the "`vv`" and "`VV`" types by placing a spacer within their columns—thus, they can be used to generate two single, or double, vertical rules whose separation distance is programmable.

The "`h`" and "`H`" types produce single and double horizontal rules, respectively. Horizontal rule types are not normally used in the column specifications, but rather with the `\IEEEeqnarraymulticol` command in order to draw a horizontal rule across one or more column(s).

Please be aware that the line commands of other alignment environments may not work properly within the IEEEeqnarray family which provides its own ways of doing these types of things. In particular, `\cline` is totally incompatible—users should use the `\IEEEeqnarraymulticol {num_cols}{h}{}` command instead. However, `\vline` `\hline` should work—unless another LaTeX package redefines them in some incompatible way. The IEEEeqnarray family provides its own version of `\vline`:

`\IEEEeqnarrayvrule[`*`rule_thickness`*`]`

which produces a vertical rule extending from the top to bottom of a cell without overriding the column type. The optional argument is for specifying the rule thickness which defaults to `\arrayrulewidth` if no argument is provided.

The IEEEeqnarray row commands (discussed in the next section) provide some alternatives to `\hline`.

### F.12 Row Commands

The IEEEeqnarray family has several commands that can be used to produce special rows which span all the columns. Unless otherwise noted, the commands described here must issued as the very first command in a given row.

To produce a spacer row which relies on the strut system, use

`\IEEEeqnarrayseprow[`*`height`*`][`*`decl`*`]`

The first argument specifies the height of the strut row, if left blank or empty, the default value of `0.25\normal baselineskip` will be assumed. The second optional argument is for commands which will be executed prior to the evaluation of the first argument as is done with `\IEEEeqnarraystrutsize`. `\IEEEeqnarrayseprow` will *not* interrupt the column definitions, so it will not cut vertical lines. If column definition suspension is desired, use the

[12] Those familiar with TeX may be interested to know that TeX's `\omit`, `\span`, and `\multispan` should work in `\IEEEeqnarraybox`, but not in `\IEEEeqnarray` because of the need to track column usage with a hidden counter.

cutting form which will override all the column types in the entire row:

\IEEEeqnarrayseprowcut[*height*][*decl*]

To produce a horizontal rule row, use:

\IEEEeqnarrayrulerow[*rule_thickness*]

which will override all the column definitions with one that produces a horizontal rule. If the optional rule thickness is not specified, the value of \arrayrulewidth will be used.

To produce a double rule row, use:

\IEEEeqnarraydblrulerow[*rule_thickness*][*spacing*]

which will produce a rule row, a (noncutting) separation row, followed by another rule row. If the optional rule thickness is not specified, the value of \arrayrulewidth will be used when producing each of the two rule rows. If the optional separation distance is not specified, the value of \doublerulesep will be used. There is also a cutting form:

\IEEEeqnarraydblrulerowcut[*rule_thickness*][*spacing*]

which works the same way except that the separation row will override all the column definitions. (Vertical rule columns will not appear inside the double rule row produced by this command.)

### F.13 Useful Low Level TeX Commands

Although the use of lower level TeX commands is generally frowned upon in LaTeX, some of them are just too helpful to ignore.

\phantom{} produces an invisible box with the width, height and depth of its contents, but the contents themselves will not appear in the output. There is also the \hphantom{} and \vphantom{} forms which retain only the contents' width, or its height and depth, respectively. As an example, look carefully at the footnotes at the bottom of the Predefined Column Separation Table 5. This table was produced using the \IEEEeqnarraybox command. The footnotes are actually contained within the last two rows of the table. Note how the left sides of the footnotes line up, even though the first one has a superscript asterisk for a footnote symbol. The reason that the second row lines up is because, at its left side, it employs a horizontal phantom of the very same symbol:

```
\hphantom{\textsuperscript{*}}
```

Vertical phantoms can be used to equalize row height or spacing—such as to get matrices that fit within brackets of the same size even though one has "tall" symbols and the other not.

The opposite of \hphantom{} is \rlap{} which displays its contents, but with zero width. There is also an \llap{} which does the same thing, but the contained object will appear just to the left of the given point, rather than after as with \rlap. For example, look closely at the first "Width" column heading in the same table. The word "Width" is centered irrespective of the asterisk. That is because the width of the asterisk was zeroed:

```
Width\rlap{\textsuperscript{*}}
```

The vertical analog of \rlap is \smash{} which reduces the apparent height and depth of its contents to zero. (LaTeX's \raisebox{0pt}[0pt][0pt]{} does about the same thing, and also provides an adjustable vertical offset.) \smash can be used when space is already reserved for an object, but that LaTeX does not "know" this and would allocate unwanted additional vertical space. One good use of smash for table objects that are to be "slipped" into a hidden row of zero height, or into a row which is to be no higher than the "short" things, such as horizontal rules, that are in its other columns.

The TeX \noalign{} command can be used within IEEEeqnarray family to inject text which is outside of the alignment structure. For example,

```
\begin{IEEEeqnarray}{rCl}
A_1&=&7\IEEEyessubnumber\\
A_2&=&b+1\IEEEyessubnumber\\
\noalign{\noindent
and\vspace{\jot}}A_3&=&d+2\IEEEyessubnumber%
\end{IEEEeqnarray}
```

When employed, \noalign must be the *very* first command in a row—even before any \IEEEeqnarraymulticol, \IEEEeqnarrayomit, or row commands.

Be forewarned that the proper use of \noalign can be tricky. There are three potential issues. 1) Remember that \noalign will place its contents outside of the alignment. So, the line spacing controls of the IEEEeqnarray commands will not be in effect. The user may have to manually add \baselineskip and/or \jot spacing as needed (which was done in the previous example). 2) Furthermore, \noalign does *not* automatically place its contents within a box. However, nonaligned material *must* be placed within a *horizontal* box when within the vertical box produced by the \IEEEeqnarraybox command. Therefore, when using \noalign within a \IEEEeqnarraybox, be sure to wrap things up in an \hbox{}:[13]

```
\noalign{\hbox{and therefore}}
```

3) Finally, there may be some issues related to how easily page breaks occur around the \noalign lines. This is only an issue with \IEEEeqnarray because page breaks cannot occur within the box produced by \IEEEeqnarraybox. If needed, page break desirability can be altered by manually entering \pagebreak, or \nopagebreak, etc., at the end of the \noalign contents.

---

[13] LaTeX's \mbox will *not* work.

## F.14 More Practical Examples of Use

The use of the IEEEeqnarray is somewhat complicated. However, once the building blocks and core concepts are understood, the user may find that is easier to use the IEEEeqnarray family for just about every alignment situation rather than to have to remember all the interfaces and unique behaviors of many different tools.

A few "real world" examples will now be demonstrated.

### *F.14.1 IEEEeqnarray Cases Structures*

Cases structures can be obtained using `\IEEEeqnarraybox`:

```
\begin{equation}
\setlength{\nulldelimiterspace}{0pt}
|x|=\left\{\begin{IEEEeqnarraybox}[\relax][c]{
l's}
x,&for $x \geq 0$\\
-x,&for $x < 0$%
\end{IEEEeqnarraybox}\right.
\end{equation}
```

Note the use of the large `\quad` (1em) spacing before the conditional statements. The zeroing of `\nulldelimiterspace`, an optional step, eliminates the width of the nonvisible closing brace "`\right.`" in order to perfectly center the visible portion of the equation.[14]

Note that both branches share a common equation number. If an equation (sub)number is wanted for each branch, the preferred solution is to use the cases.sty package as discussed in the Section 8.1. However, it is possible to use \IEEEeqnarray to build such a thing—although it takes extra work and a few tricks to do so. For example,

```
\begin{IEEEeqnarray}[\setlength{\nulldelimiter
space}{0pt}]{rl's}
&x,&for   $x   \geq   0$\IEEEyessubnumber\\*[-
0.625\normalbaselineskip]
\smash{|x|=\left\{\IEEEstrut[3\jot][3\jot]\rig
ht.}&&
\nonumber\\*[-0.625\normalbaselineskip]
&-x,&for $x < 0$\IEEEyessubnumber
\end{IEEEeqnarray}
```

A hidden middle row is used to hold the left hand side of the equality. In order to prevent this row from altering the spacing between the two branches, its height must be smashed and the extra line spacing (which consists of `\baselineskip`, plus `\jot` which is normally `0.25\baselineskip` for IEEEtran.cls.) must be removed, half from above and half from below—Making it look as though the middle row never occurred. Because the large brace cannot "see" the height of the branches, it must be manually sized with a strut. The star form of the new line commands is used to prevent the possibility of a page break within the structure.

[14] The width of null delimiters is typically only 1.2pt, and so can usually be safely ignored.

### *F.14.2 Matrices*

Displayed matrices can easily be created with `\IEEEeqnarraybox`:

```
\begin{equation}
I                                            =
\left(\begin{IEEEeqnarraybox*}[][c]{,c/c/c,}
1&0&0\\
0&1&0\\
0&0&1%
\end{IEEEeqnarraybox*}\right)
\end{equation}
```

Because the example matrix has elements of normal height, one can use the star form of `\IEEEeqnarraybox` to turn off the extra `\jot` component of the line spacing so as to make a more compact matrix. If larger symbols had been used in the matrix, the nonstar form would be the better choice. `\arraycolsep` typically serves quite well as an element column separator. A standard small math space is added to the ends of the matrix to provide a little distance between it and its enclosing parentheses.

It is instructive to show how to construct a "small" matrix:[15]

```
\newcommand{\mysmallarraydecl}{%
\renewcommand{\IEEEeqnarraymathstyle}{\scripts
criptstyle}%
\renewcommand{\IEEEeqnarraytextstyle}{\scripts
ize}%
\renewcommand{\baselinestretch}{1.1}%
\settowidth{\normalbaselineskip}{\scriptsize
\hspace{\baselinestretch\baselineskip}}%
\setlength{\baselineskip}{\normalbaselineskip}
%
\setlength{\jot}{0.25\normalbaselineskip}%
\setlength{\arraycolsep}{2pt}}
%
\begin{equation}
S=\left[\begin{IEEEeqnarraybox*}[\mysmallarray
decl]
[c]{,c/c,}
1/2&0\\
0&3/4%
\end{IEEEeqnarraybox*}\right]
\end{equation}
```

The use of a user defined command, `\mysmallarraydecl`, to contain the IEEEeqnarray setup code, demonstrates how users can easily recreate their most commonly used structures by fully exploiting the on-the-fly configurability of the IEEEeqnarray family.

This example is more complex than need be in order to demonstrate a few techniques. It would be easy enough to set `\baselineskip` to the desired value, but suppose that

[15] IEEE authors should note that the use of small matrices is not recommended as IEEE does not usually reduce font sizes in equations or alter the main text baselineskip to accommodate in-text mathematics.

TABLE 6
Network Delay as a Function of Load

| $\beta$ | Average Delay | |
|---|---|---|
| | $\lambda_{min}$ | $\lambda_{max}$ |
| 1 | 0.057 | 0.172 |
| 10 | 0.124 | 0.536 |
| 100 | 0.830 | 0.905* |

*limited usability

the matrix rows are to be spaced some multiple of the `\baselineskip` of the `\scriptsize` font. Complicating matters even more is the fact that most LaTeX class files will not allow the user to execute text font size commands within math mode—and the matrix is within an equation. So, `\scriptsize` cannot be used to directly set the `\baselineskip`.

The first step is to set the math and text columns to their desired styles. Then, `\baselinestretch` is setup to be used like `\arraystretch`. The trick is to run `\scriptsize` within a `\settowidth` command which stores the `\baselineskip` of the `\scriptsize` font, multiplied by `\baselinestretch`, in `\normalbaselineskip` which is then used to set `\baselineskip`, `\jot`, etc. Finally, `\arraycolsep` is reduced to better suit the smaller font. Note the use of "`%`" to prevent unwanted spaces from appearing after the braces at the end of lines in `\mysmallarraydecl`.

### F.14.3 Tables

Tables, especially those with lines, tend to be a little more complicated. Table 6 was made with the following code:

```
\begin{table}
\centering
\caption{Network Delay as a Function of Load}
\label{table_delay}
\begin{IEEEeqnarraybox}[\IEEEeqnarraystrutmode
\IEEEeqnarraystrutsizeadd{2pt}{0pt}]
{x/r/Vx/r/v/r/x}
\IEEEeqnarraydblrulerowcut\\
&&&&\IEEEeqnarraymulticol{3}{t}{Average De-
lay}&\\
&\hfill\raisebox{-
3pt}[0pt][0pt]{$\beta$}\hfill&&
\IEEEeqnarraymulticol{5}{h}{}%
\IEEEeqnarraystrutsize{0pt}{0pt}\\
&&&&\hfill\lambda_{\mbox{min}}\hfill&&\hfill
\lambda_{\mbox{max\vphantom{i}}}\hfill&
\IEEEeqnarraystrutsizeadd{0pt}{2pt}\\
\IEEEeqnarraydblrulerowcut\\
&1&&&   0.057&& 0.172&\\
&10&&&  0.124&& 0.536&\\
&100&&&                                0.830&&
0.905\rlap{\textsuperscript{*}}&\\
\IEEEeqnarraydblrulerowcut\\
&\IEEEeqnarraymulticol{7}{s}{\scriptsize\texts
uperscript{*}limited
usability}%
\end{IEEEeqnarraybox}
\end{table}
```

Because this table has lines, the first step is to enable strut mode line spacing. The strut height is then increased by a couple of points to provide a little more headroom above the letters.[16] This table uses cutting horizontal rules and open sides as is commonly done in IEEE publications. There are three extra "x" columns which serve as place holders. The "x" columns at each end serve as a quick way to get the horizontal rules to extend a little past the contents of the table. The middle "x" column serves as an attachment point for the horizontal rule that is below "Average Delay." Without this extra column, the left side of that horizontal rule would cut into the middle double vertical rule.[17] Notice how the "$\beta$" is smuggled in as part of the row containing the horizontal rule. $\beta$ has to be smashed so that it will not add unwanted vertical spacing. Likewise, the strut for that row is disabled. Also, `\raisebox` is used instead of `\smash`, so that $\beta$ can be vertically lowered—otherwise, it would appear on its baseline which is too high for the purpose at hand. The `\hfill` on either side of $\beta$ changes the justification of that cell to centered. The "min" and "max" subscripts would not normally sit at the same level because the "i" in min is slightly higher than the letters in "max." To fix this, a `\vphantom` "i" is added to "max." Because these subscripts sit so low, the depth of that line's strut is increased a couple of points. Alternatively, one could have just smashed the "i." The asterisk next to "0.905" is reduced to zero width via `\rlap` so that it will not affect its cell's width or alignment. This example also illustrates how to integrate table footnotes into the end of a table without the help of external packages.

Strut spacing does not work so well for rows that contain tall symbols because such objects routinely exceed the height of the struts. Furthermore, increasing the strut height is often not an option because 1) the height and depth of the tall symbols must be measured or guessed and 2) there may be other rows which have normal line height. The code in Table 7 illustrates such a situation. Its code is as follows:

```
\begin{table}
\centering
\caption{Possible $\Omega$ Functions}
\label{table_omega}
\begin{IEEEeqnarraybox}[\IEEEeqnarraystrutmode
\IEEEeqnarraystrutsizeadd{2pt}{1pt}]%
{v/c/v/c/v}
\IEEEeqnarrayrulerow\\
&\mbox{Range}&&\Omega(m)&\\
\IEEEeqnarraydblrulerow\\
\IEEEeqnarrayseprow[3pt]\\
```

[16] Knuth calls this extra step a mark of quality.
[17] Some may even think it would be better that way, but we want to show some tricks in these examples.

TABLE 7
Possible $\Omega$ Functions

| Range | $\Omega(m)$ |
|---|---|
| $x < 0$ | $\Omega(m) = \sum\limits_{i=0}^{m} K^{-i}$ |
| $x \geq 0$ | $\Omega(m) = \sqrt{m}$ |

```
&x < 0&&\Omega(m)=\sum\limits_{i=0}^{m}K^{-i}&
\IEEEeqnarraystrutsize{0pt}{0pt}\\
\IEEEeqnarrayseprow[3pt]\\
\IEEEeqnarrayrulerow\\
\IEEEeqnarrayseprow[3pt]\\
&x                                        \ge
0&&\Omega(m)=\sqrt{m}\hfill&\IEEEeqnarraystrut
size{0pt}{0pt}\\
\IEEEeqnarrayseprow[3pt]\\
\IEEEeqnarrayrulerow
\end{IEEEeqnarraybox}
\end{table}
```

The solution is to use `\IEEEeqnarrayseprow` to manually add in a fixed amount of extra space as needed. In this way, `\IEEEeqnarrayseprow` can do for lined tables what `\jot` does for multiline equations. Of course, using this method, the baselines of the rows will no longer be equally spaced.

The `\hfill` in the square root cell is a cheap, but effective, way of getting the equal signs to line up without the need of additional columns.
