# Supplementary material for: DPCube: Differentially Private Histogram Release through Multidimensional Partitioning
Source: arXiv:1202.5358 source file (2012-02-24)
Supplement: Supplementary file 2 [file Appendix.tex]

\section{Proof of Theorem \ref{theo-adverarial}}
\label{app-proof-adversarial}
\begin{proof}
\begin{align*}
Pr[D|A_1,A_2]=\frac{Pr[A_1,A_2|D]}{Pr[A_1,A_2]}\\
=\frac{Pr[A_2|D]\cdot Pr[A_1|D]\cdot Pr[D]}{Pr[A_1,A_2]}\\
=\frac{Pr[A_2|D]\cdot Pr[D|A_1]\cdot Pr[A_1]}{Pr[A_2]\cdot Pr[A_1]}\\
=\frac{Pr[A_2|D]\cdot Pr[D|A_1]}{Pr[A_2]}
\end{align*}

Let's recap the model of differential privacy. Assume the attacker knows all the record except the $i$th record $d_i$.
Let $q_l$ be the $l$th query, $Q(q_l)$ be the true answer of $q_l$, $a_l$ be the perturbed answer of $q_l$.
Let $x$ be the range of $d$, $D$ be the event that $d_i=x_1$,
$P_l$ be the posterior probability of $Pr[D|a_1, a_2,\cdots a_l]$.
Let $A_1=\{a_1, a_2,\cdots ,a_{l-1}\}$, $A_2=\{a_l\}$, then
\begin{align*}
P_l=Pr[D|A_1,A_2]=P_{l-1}\cdot \frac{Pr[A_2|D]}{Pr[A_2]}\\
=P_{l-1}\cdot \frac{Pr[a_l|d_i=x_1]}{\sum_{x_j\in x}Pr[a_l|d_i=x_j]\cdot Pr[d_i=x_j]}
\end{align*}
If we adopt Laplace noise to achieve differential privacy, then

\begin{align*}
\frac{p_l}{p_{l-1}}=\frac{\frac{1}{2b}exp(-|a_l-Q(q_l,x_1)|/b)}{\sum_{x_j\in x}\frac{1}{2b}exp(-|a_l-Q(q_l,x_j)|/b)\cdot Pr[d_i=x_j]}\\
%=\frac{1}{\sum_{x_j\in x} exp(-(|a_l-Q(q_l,x_j)|-|a_l-Q(q_l,x_1)|)/b)\cdot Pr[d_i=x_j]}\\
\leq \frac{1}{\sum_{x_j\in x} exp(-|Q(q_l,x_j)-Q(q_l,x_1)|/b)\cdot Pr[d_i=x_j]}
\end{align*}
Recall the definition of S, then
\begin{align*}
|Q(q_l,x_j)-Q(q_l,x_1)|\leq S
\end{align*}
\begin{align*}
\frac{P_l}{P_{l-1}}\leq \frac{1}{\sum_{x_j\in x} exp(-S/b)\cdot
Pr[d_i=x_j]}
\end{align*}
Because $b=S/\alpha$, then
$
P_l/P_{l-1}\leq e^\alpha
$.
So, $Pr[V=d]\leq P_0*exp({l\alpha})$.
\end{proof}
